# Supplementary material for: Phenomena in Gravitational Clustering
Source: arXiv:astro-ph/0509251 source file (2005-09-09)
Supplement: Supplementary file 1 [file appendixA.tex]

\section{Appendix A. On NBODY simulations}

The NBody simulations referred to in this thesis are dark matter simulations performed with a Particle Mesh code written by Dr. Jasjeet Singh Bagla (jasjeet@mri.ernet.in). As far as N body simulations go there are different classes of algorithms and a variety of initial conditions which are examined using these simulations. The data analysis part of NBody simulations depends on the aspect of the problem that is being studied. Nevertheless it is possible to envisage an integrated framework for NBody simulations in the lines of observational data models. 
\par
NBody simulations are to be considered as data against which theories and observations can be compared. In this model, a simulation is seen as a data source just like an object in the sky. In analogy with the fact that multi wavelength observations of an object mandates different data storage and processing strategies for different wavelengths
